# Supplementary material for: Devising a Set of Compact and Explainable Spoken Language Feature for Screening Alzheimer's Disease
Source: arXiv:2411.18922 source file (2024-11-28)
Supplement: Supplementary file 1 [file Appendix.tex]

\appendix
\clearpage
\section{Appendix}
\label{sec:appendix}

\subsection{Keyword Sets}
\label{sec:appendix-kwset}
By leveraging the human prior knowledge of Cookie Theft picture and the advanced linguistic ability of LLMs, we propose the following keyword sets:
\begin{itemize}
    \item Keyword set 0: "boy", "reach", "stool", "tip", "grab", "stand", "jar"
    \item Keyword set 1: "girl", "look", "stand", "floor", "worried", "smile"
    \item Keyword set 2: "mother", "mom", "wash", "sink", "busy", "turn"
    \item Keyword set 3: "water", "soap", "cupboard", "dishes", "overflowing"
    \item Keyword set 4: "counter", "window", "curtain", "light", "trees"
\end{itemize}

\subsection{Supplementary tables and figures}
\label{sec:appendix-sup}
\input{latex/Tables/description}

\begin{figure*}[!t] % The figure* environment makes the figure span two columns
    \centering
    \includegraphics[width=\textwidth]{latex/Figs/feature_importance.pdf}
    \caption{Feature importance using Random Forest classifier. The highlighted features are our proposed features. Three of our features ranked at Top 5 and six of them ranked at top 10.}
    \label{fig:feature_importance}
\end{figure*}

\input{latex/Tables/correlation}

\begin{figure*}[!t] % The figure* environment makes the figure span two columns
    \centering
    \includegraphics[width=\textwidth]{latex/Figs/topic_feature_distribution.pdf}
    \caption{Topic features value distribution.}
    \label{fig:topic_feature_dist}
\end{figure*}

\begin{figure*}[!t] % The figure* environment makes the figure span two columns
    \centering
    \includegraphics[width=\textwidth]{latex/Figs/GPT_feature_distribution.pdf}
    \caption{LLM based features value distribution.}
    \label{fig:GPT_feature_dist}
\end{figure*}

\begin{figure*}[!t]
    \centering
    \includegraphics[width=1.0\textwidth]{latex/Figs/stability_whisper.png}
    \caption{Comparison of Feature Stability Using Different ASR transcription for AD Detection}
    \label{fig:steability}
\end{figure*}
\input{latex/Tables/prompts}
